# Supplementary material for: Randomized Smoothing with Masked Inference for Adversarially Robust Text Classifications
Source: arXiv:2305.06522 source file (2023-05-11)
Supplement: Supplementary file 1 [file inference_time.tex]

\section{Run time analysis}
\begin{wraptable}{r}{0.55\linewidth}
	\caption{Run time comparison of RSMI with the baselines.}
	\label{table:computation_time}
	\centering
 	\scalebox{0.90}{
	\begin{tabular}{llcccccccccc}
	\toprule
	Dataset & Model & Train ($\downarrow$) & Inference ($\downarrow$)\\
	\midrule
	\multirow{6}{*}{QNLI}
	& RoBERTa-base    &  & \\
	& + Fine-Tuned     & \ \,\,1.0  & \ \,\,1.0  \\ 
	& + FreeLB\free   & $\times$2.8 & $\times$1.0   \\ 
	& + InfoBERT\info & $\times$5.4 & $\times$1.0   \\ 
	& + SAFER\safer   & $\times$1.0 & $\times$1.0 \\ 
	& + RSMI (Our)    & $\times$1.9 & $\times$3.5   \\ 
	\bottomrule
	\end{tabular}
 	}
\end{wraptable}
We compared the speed of RSMI with baseline algorithms on the RoBERTa-base model. The training speed of each algorithm is evaluated on the training set of QNLI dataset and the dev set of QNLI dataset is used for an inference speed analysis. All of the experiments are conducted on an Intel Xeon Gold 5218R CPU-2.10GHz processor with a single Quadro RTX 6000 GPU under Python with PyTorch. \Cref{table:computation_time} summarizes the run time analysis experiments. RSMI is approximately 1.9 times slower than the Fine-Tuned model in training and 3.5 times slower than the inference speed of the Fine-Tuned model. The latency of RSMI is mainly caused by the additional backward propagation and forward propagation for computing gradients (\cf Algorithm 1). Note that for a fair comparison, we set the number of gradient computation steps of FreeLB and InfoBERT at 3.
